# Supplementary material for: An alternating peak-optimization method for optimal trajectory generation of quadrotor drones
Source: arXiv:2312.02944 source file (2023-12-05)
Supplement: Supplementary file 1 [file FlownTrajectories.tex]

\begin{figure}[h!]
    \centering
    \includegraphics[width=0.48\textwidth]{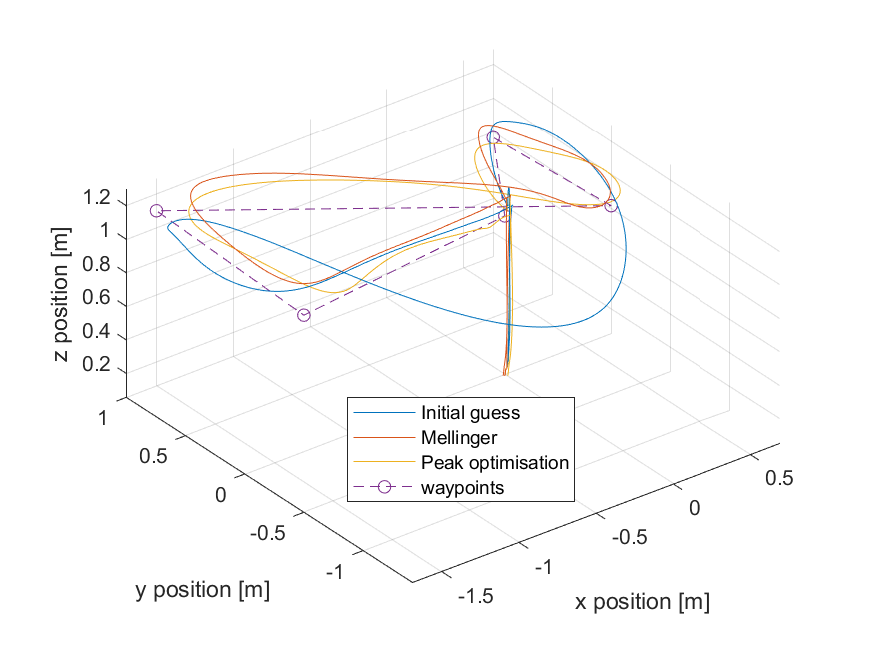}
    \caption{Measured minimum snap trajectories in 3D-space}
    \label{fig:Exp_Snap_XYZ}
\end{figure}

\begin{figure}[h!]
    \centering
    \includegraphics[width=0.48\textwidth]{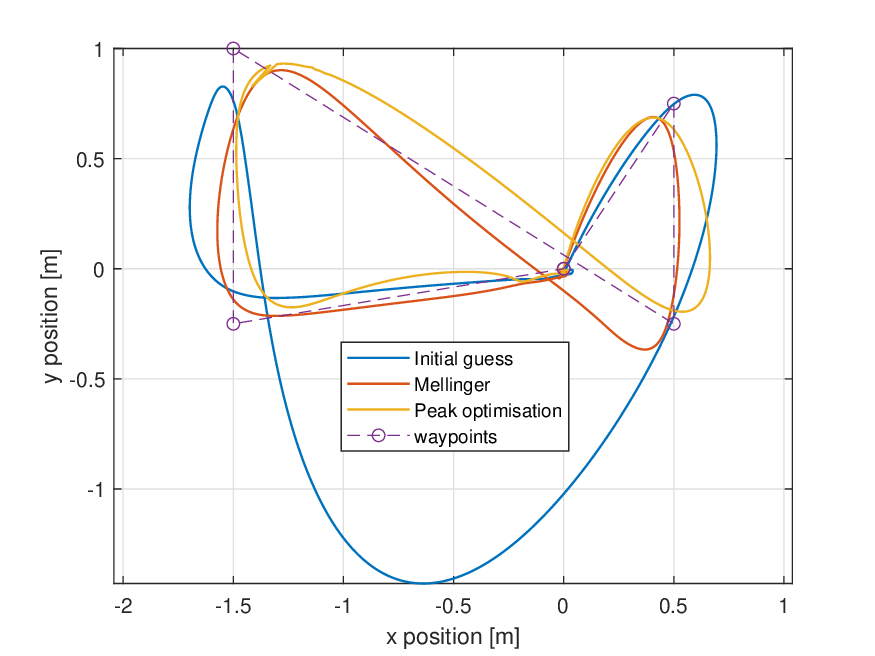}
    \caption{Measured minimum snap trajectories in the XY-plane}
    \label{fig:Exp_Snap_XY}
\end{figure}

\begin{figure}[h!]
\hspace*{-0.7cm}   
    \centering
    \includegraphics[width=0.55\textwidth]{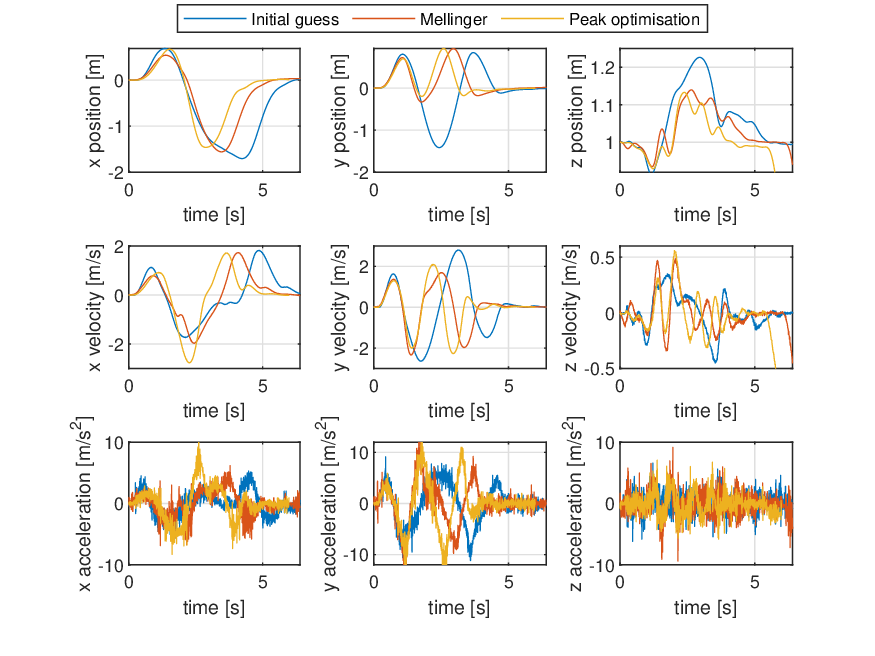}
    \caption{Higher order dynamics of the minimum snap trajectories measurements}
    \label{fig:Exp_Snap_XYZ_der}
\end{figure}

\begin{figure}[h!]
    \centering
    \includegraphics[width=0.48\textwidth]{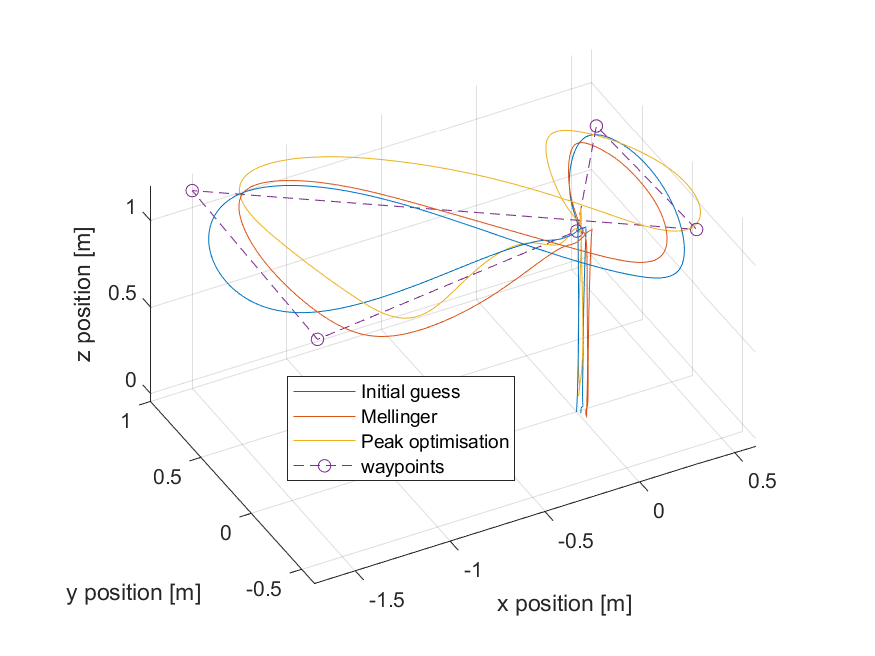}
    \caption{Measured minimum jerk trajectories in 3D-space}
    \label{fig:Exp_jerk_XYZ}
\end{figure}

\begin{figure}[h!]
    \centering
    \includegraphics[width=0.48\textwidth]{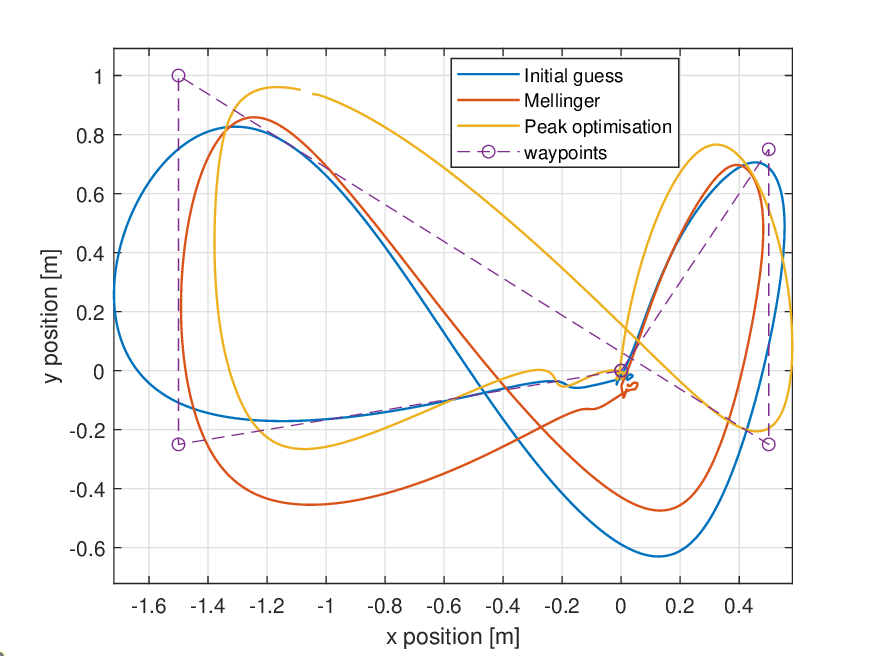}
    \caption{Measured minimum jerk trajectories in the XY-plane}
    \label{fig:Exp_jerk_XY}
\end{figure}

\begin{figure}[h!]
\hspace*{-0.7cm}   
    \centering
    \includegraphics[width=0.55\textwidth]{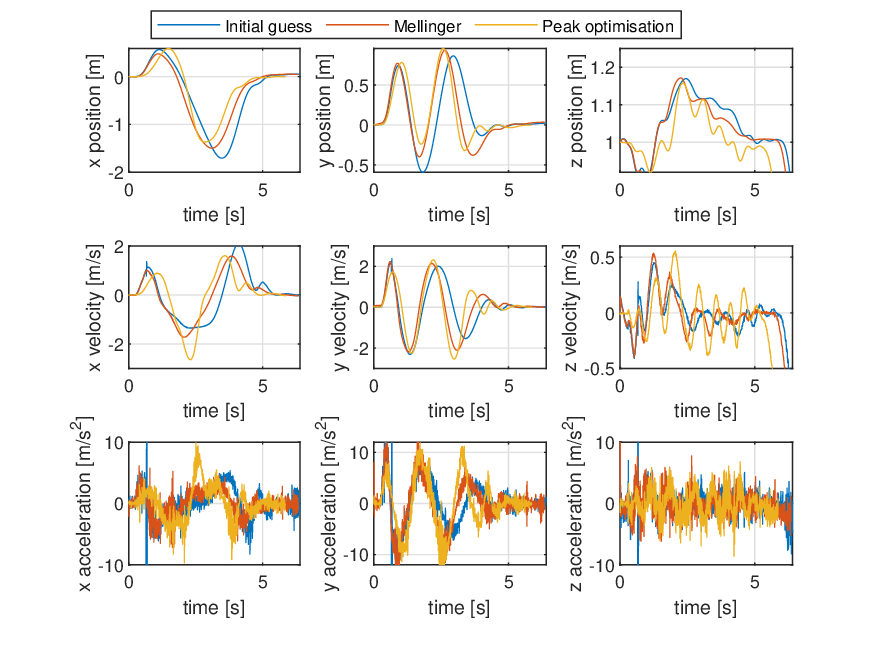}
    \caption{Higher order dynamics of the minimum jerk trajectories measurements}
    \label{fig:Exp_jerk_XYZ_der}
\end{figure}
