# Supplementary material for: An alternating peak-optimization method for optimal trajectory generation of quadrotor drones
Source: arXiv:2312.02944 source file (2023-12-05)
Supplement: Supplementary file 2 [file Acknowledgments.tex]

I would like to thank dr. Zhiyong Sun for his guidance and answers during this project. Furthermore I would like to thank Canye Wang for answering all my questions regarding the Crazyswarm system and for allowing me to use his polynomial coefficient optimisation code and helping me rewrite it to work with the Crazyswarm system.
