# Supplementary material for: An alternating peak-optimization method for optimal trajectory generation of quadrotor drones
Source: arXiv:2312.02944 source file (2023-12-05)
Supplement: Supplementary file 3 [file ExtendedBEP.tex]

The extended literature review can be found in \autoref{Chapters:DiffFlat} and the extra work for the BEP was the implementation in the real drones as described in \autoref{Chapters:Results}.
