# Supplementary material for: An alternating peak-optimization method for optimal trajectory generation of quadrotor drones
Source: arXiv:2312.02944 source file (2023-12-05)
Supplement: Supplementary file 4 [file Parameters.tex]

\begin{table}[h!] 
\centering
\caption{Parameters used during experiments}
\label{table:param}
\begin{tabular}{  m{1.5cm} | m{2cm}| m{0.75cm} | m{1cm} | m{1.5cm}  } 

Jerk or Snap optimisation method & segment times optimisation method  & Initial total time & Temporal scaling & Maximum jerk $J_{max}$ \\ 
\hline
Snap & Initial guess & 10 s & 55.0\% & -  \\\hline
Snap & Mellinger method & 10 s & 47.5\% & - \\\hline
Snap & Peak optimisation method & 10 s & 100\% & 40 $m/s^3$   \\\hline
Jerk & Initial guess & 10 s & 45\% & -\\\hline
Jerk  & Mellinger method & 10 s & 43.5\% & -\\\hline
Jerk & Peak optimisation method & 10 s & 97.5\% & 50 $m/s^3$ \\\

\end{tabular}
\end{table}
