# Supplementary material for: An alternating peak-optimization method for optimal trajectory generation of quadrotor drones
Source: arXiv:2312.02944 source file (2023-12-05)
Supplement: Supplementary file 5 [file Properties.tex]

\begin{table}[h!] 
\centering
\caption{System properties of Crazyflie 2.1}
\begin{tabular}{c|c|c}

Property & Value & Unit \\ 
\hline
mass & 0.031 & $[kg]$   \\
$I_x$ & 17.5617 & $10^{-6} [kg m^2]$   \\
$I_y$ & 17.6456 & $10^{-6} [kg m^2]$   \\
$I_z$ & 30.2517 & $10^{-6} [kg m^2]$  \\
$d$   & 0.04  & $[m]$ \\
$k_F$ & 0.005022 & $[N s^2]$ \\
$k_M$ & 1.8580 & $10^{-5} [N m s^2]$ \\

\end{tabular}

\label{table:1}
\end{table}
