# Supplementary material for: An alternating peak-optimization method for optimal trajectory generation of quadrotor drones
Source: arXiv:2312.02944 source file (2023-12-05)
Supplement: Supplementary file 6 [file SimuFig.tex]

\begin{figure}[h!]
    \centering
    \includegraphics[width=0.48\textwidth]{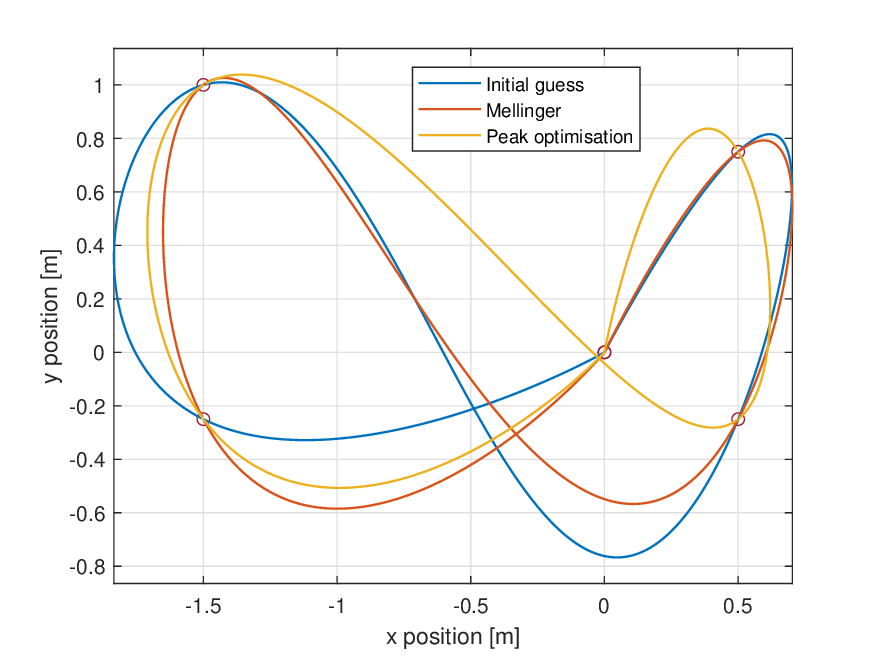}
    \caption{Minimum jerk trajectories}
    \label{fig:JerkXY}
\end{figure}

\begin{figure}[h!]
\hspace*{-0.5cm}
    \centering
    \includegraphics[width=0.5\textwidth]{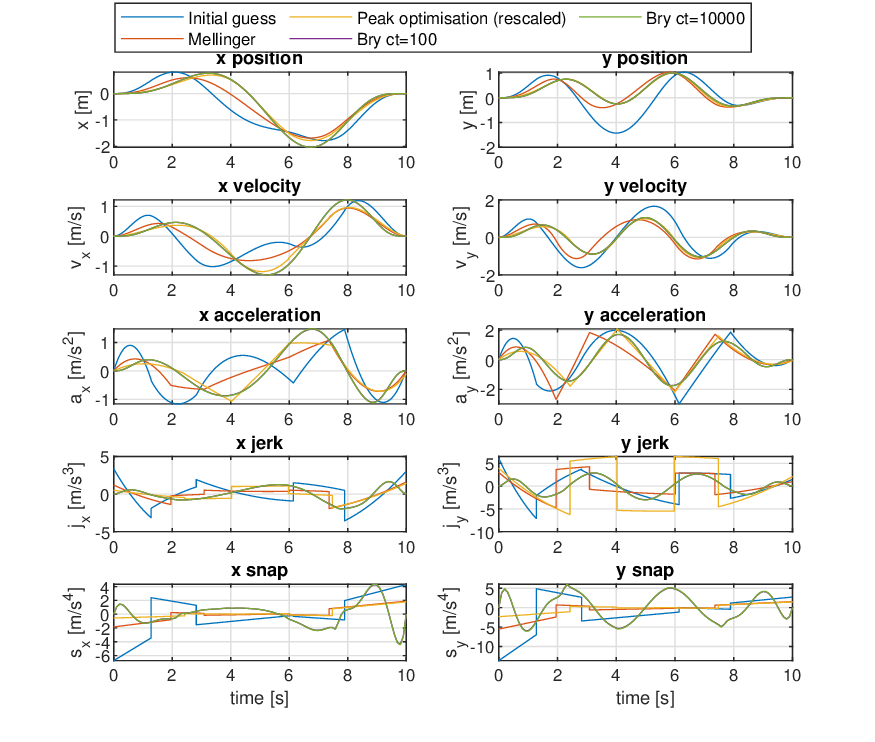}
    \caption{Higher order dynamics of generated minimum snap trajectories}
    \label{fig:Snapder}
\end{figure}

\begin{figure}[h!]
\hspace*{-0.5cm}
    \centering
    \includegraphics[width=0.5\textwidth]{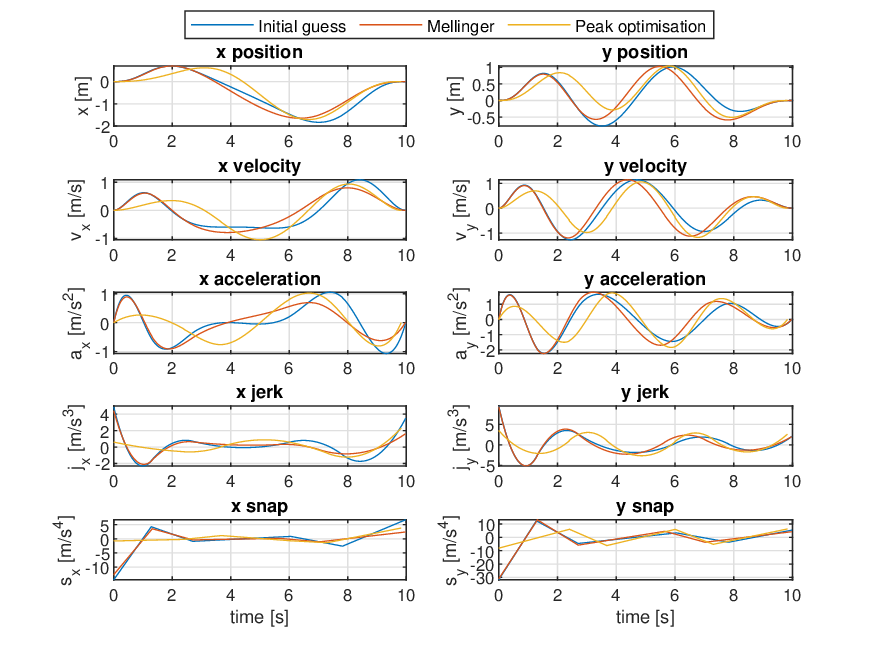}
    \caption{Higher order dynamics of generated minimum jerk trajectories}
    \label{fig:Jerkder}
\end{figure}
